# Supplementary material for: Identification of a Griffiths singularity in a geometrically frustrated antiferromagnet
Source: arXiv:1609.03812 source file (2016-09-13)
Supplement: Supplementary file 1 [file Supple.pdf]

# Supplementary materials for "Identification of a Griffiths singularity in a geometrically frustrated antiferromagnet"

Jitender Kumar,[1] Soumendra Nath Panja,[1] Shanu Dengre,[1] and Sunil Nair[1,2]

[1]*Department of Physics, Indian Institute of Science Education and Research*
[2]*Centre for Energy Science, Indian Institute of Science Education and Research,*
*Dr. Homi Bhabha Road, Pune, Maharashtra-411008, India*

(Dated: September 13, 2016)

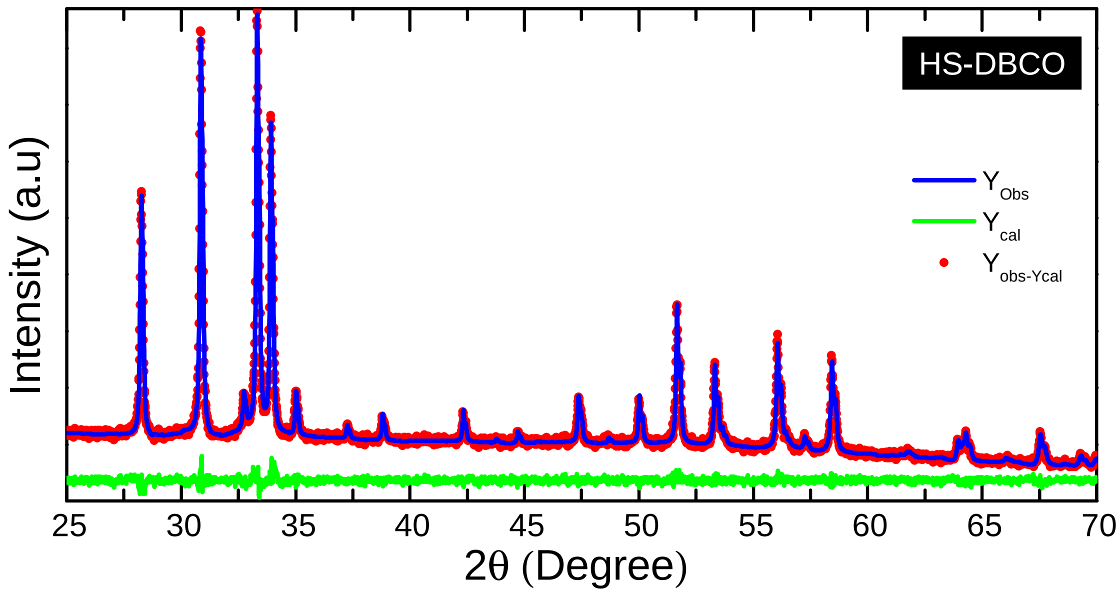


Fig.S1:Rietveld refinement of the room temperature XRD data of the HS-DBCO specimen

Table I: Structural parameters as obtained from Rietveld refinement of $DyBaCo_4O_{7.12}$ (HS-DBCO) at $T = 300K$ ; Space Group : $P31c$, Crystal system: Trigonal , Unit cell parameters a = b = 6.311(65) Å,c = 10.241(48) Å, $\alpha$ = $\beta$ = 90 °,$\gamma$ = 120 °

| Atom | Wyckoff | x/a | y/b | z/c |
|---|---|---|---|---|
| Dy | 2b | 0.66(670) | 0.33330 | 0.87(218) |
| Ba | 2b | 0.66(670) | 0.33330 | 0.50000 |
| Co1 | 2a | 0.00000 | 0.00000 | 0.44(481) |
| Co2 | 6c | 0.15(750) | 0.81(500) | 0.68(590) |
| O1 | 6c | 0.51(231) | 0.50(531) | 0.75(266) |
| O2 | 2a | 0.00000 | 0.00000 | 0.24(440) |
| O3 | 6c | 0.11(703) | 0.78(840) | 0.50(050) |

$DyBaCo_4O_{7+\delta}$ samples with varying stoichiometry were prepared by quenching in different media from 1150 °C . Room temperature powder X-Ray diffraction data was collected under the continuous scanning mode with a Cu $K_\alpha$ source . Rietveld refinement of HS-DBCO ($\delta$=0.12) and LS-DBCO ($\delta$=0.07) specimens are shown in Fig.S1 and Fig.S2. For all samples in this report, refinement was attempted using space groups $P63mc$ , $Pbn2_1$ ,$Pbc2_1$ ,$Pna2_1$ and $Cc$. HS-DBCO is seen to crystallize in the Trigonal $P31c$ space group, whereas LS-DBCO crystallizes in the Orthorhombic $Pna2_1$ space group.The refinement was poor for other space groups. Samples with $\delta$ = 0.23 ,0.24 ,0.26 stabilize in the $Pna2_1$ symmetry (Space Group No.33) at room temperature. Details of room temperature crystallographic unit cell parameters of LS-DBCO and HS-DBCO are given below in Table.I and Table.II . The oxygen stoichiometry of all samples have been confirmed by Idiometric titration.

With decreasing temperature the symmetry lowering transition $P31c \rightarrow Pna2_1$ of LN-DBCO is shown in Fig.S3.Two Bragg peaks [620] and [040] of the lower symmetry phase are seen to converge into a single [220] peak in the higher symmetry phase.

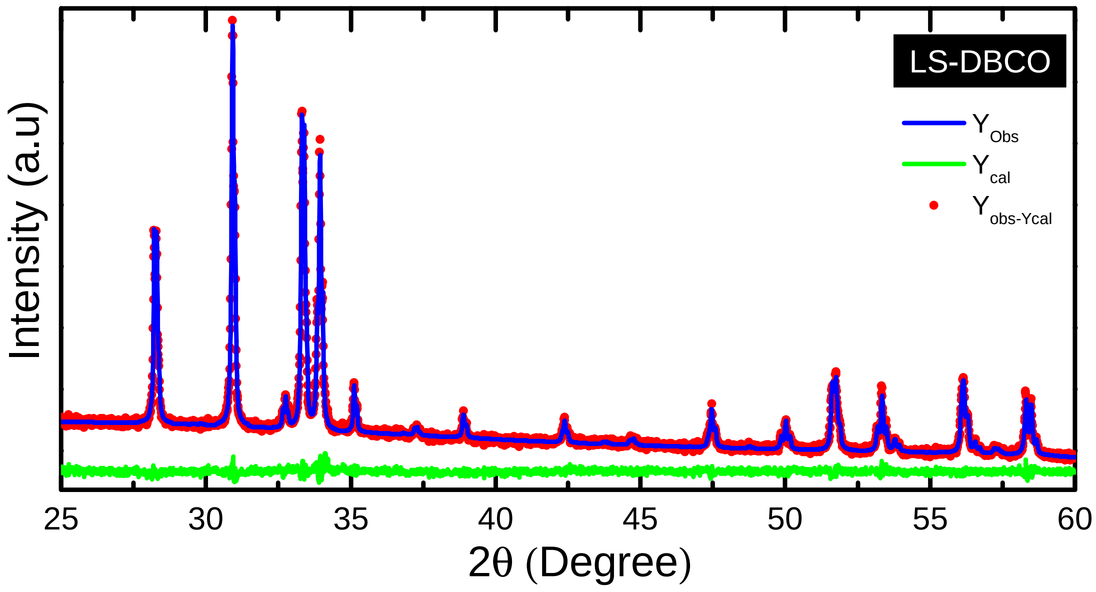


Fig.S2:Rietveld refinement of the room temperature XRD data of the LS-DBCO specimen

Table II: Structural parameters as obtained from the Rietveld refinement of $DyBaCo_4O_{7.07}$ (LS-DBCO) at $T = 300K$; Space Group : $Pna2_1$ , Unit cell parameters: a = 10.96053 Å, b = 6.30285Å,c = 10.21409Å. Crystal system: Orthorhombic, $\alpha = \beta = \gamma = 90$ °

| Atom | Wyckoff | x/a | y/b | z/c |
|---|---|---|---|---|
| Dy | 4a | 0.66(914) | 0.99(700) | 0.87(282) |
| Ba | 4a | 0.65(968) | 0.00000 | 0.49(975) |
| Co1 | 4a | 0.98(894) | 0.00000 | 0.94(338) |
| Co2 | 4a | 0.16(721) | 0.00(600) | 0.68(519) |
| Co3 | 4a | 0.08(570) | 0.75(109) | 0.18(377) |
| Co4 | 4a | 0.91(407) | 0.74(963) | 0.69(829) |
| O1 | 4a | 0.99(800 | 0.00()100) | 0.25(100) |
| O2 | 4a | 0.16(140) | 0.04(900) | 0.49(700) |
| O3 | 4a | 0.09(930) | 0.76(900) | 0.99(900) |
| O4 | 4a | 0.94(010 ) | 0.73(200) | 0.49(600) |
| O5 | 4a | 0.49(300) | 0.99(800) | 0.24(700) |
| O6 | 4a | 0.25(600) | 0.22(500) | 0.78(200) |
| O7 | 4a | 0.75(200) | 0.22(000) | 0.22(100) |

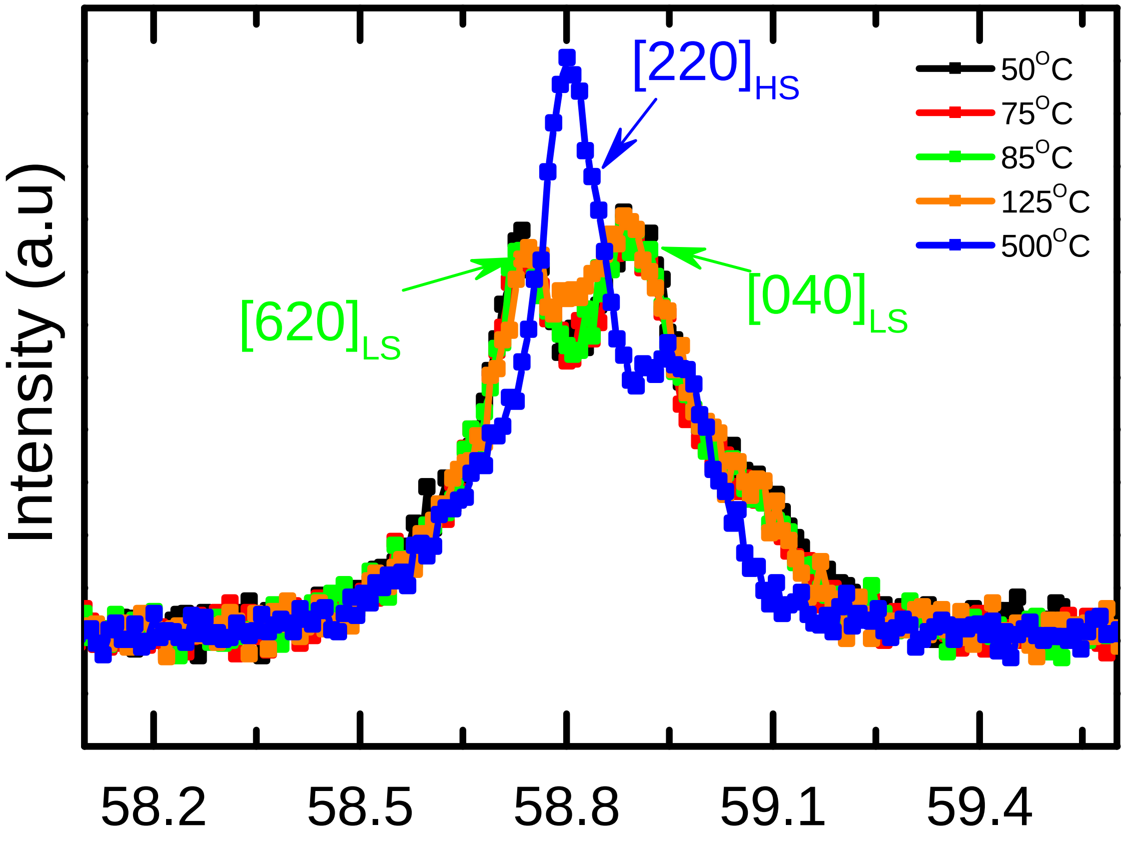


Fig.S3: Structural transition of LS-DBCO from the low symmetry $Pna2_1 \rightarrow$ high symmetry $P31c$ phase
.
